# Supplementary material for: Algorithm-driven Advances for Scientific CT Instruments: From Model-based to Deep Learning-based Approaches
Source: arXiv:2104.08228 source file (2021-09-15)
Supplement: Supplementary file 1 [file appendix.tex]

\section{Composition property of surrogate functions}
\label{app:ComPropSurrogate}

\begin{theorem}
\textit{Composition property} - Let $q(z;z^{\prime})$ be a surrogate 
function for the minimization of $t(z)$ on $\mathcal{A} \subset 
\mathbb{R}^{N}$; and let $h:\mathcal{A} \rightarrow \mathcal{A}$.  
Then define
\begin{eqnarray}
\tilde{t}(z) &\triangleq& t(h(z)) \nonumber \\
\tilde{q}(z;z^{\prime}) &\triangleq& q(h(z);h(z^{\prime})) \nonumber
\end{eqnarray}
Then $\tilde{q}(z;z^{\prime})$ is a surrogate function for 
$\tilde{t}(z)$.
\end{theorem}
\begin{proof}
The theorem can be proved by verifying the sufficiency 
coditions for surrogate functions in \eqref{eq:SubFnCond}. 
Notice that at $z=z^{\prime}$, 
$\tilde{q}(z^{\prime};z^{\prime})=\tilde{t}(z^{\prime})$ because 
$q$ is a surrogate function to $t$. Furthermore, for any 
$z \subset \mathcal{A}$, 
$\tilde{q}(z;z^{\prime}) \geq \tilde{t}(z)$ by the construction
of $q$ i.e., $q(z;z^{\prime}) \geq t(z)$ for 
$z \subset \mathcal{A}$. Therefore the compostion is still 
a surrogate function because it satisfies the sufficiency 
conditions in \eqref{eq:SubFnCond}. 
\end{proof}
